# Supplementary material for: 3D Foundation Model-Based Loop Closing for Decentralized Collaborative SLAM
Source: arXiv:2602.02430 source file (2026-02-02)
Supplement: Supplementary file 1 [file supplemental_material.tex]

\ExecuteMetaData[figures/experimentation_figures.tex]{scaling-init}

Using the loop closure inliers from our set of image pairs, we compared different scale initialization techniques, as shown in~\cref{fig:scaling-init}. We evaluated ground truth scaling, the direct approach (which uses the raw output of MASt3R), and scaling based on odometry estimates (see~\cref{eq:scaleinit}). Additionally, we compared these results with relative poses obtained using SuperPoint+SuperGlue and OpenCV (which implements Nister's method~\cite{nisterEfficientSolutionFivepoint2004} with ORB~\cite{rubleeORBEfficientAlternative2011} features and descriptors) to assess whether our scale initialization method would also benefit those approaches.

The results in~\cref{fig:scaling-init} demonstrate that our approach significantly reduces translation error for data-driven MASt3R, whereas the same improvement was not observed with the other methods. This may be explained by MASt3R's ability to output 3D point maps that are scale-consistent within a given image domain or environment. However, the mean translation error remains above 2 meters, which is high for accurate pose graph optimization. Therefore, further refinement of the scale during pose graph optimization is necessary.

\ExecuteMetaData[figures/experimentation_figures.tex]{conf-pg-boxplot}

In the following experiments, we evaluate the full pose graph solution involving all six robots from the GrAco sequence. Based on the previously mentioned feature correspondences ratio, we mapped it to a confidence metric (see~\cref{eq:confidence}), which we used to weight the inter-robot loop closures during pose graph optimization.

\cref{fig:conf-pg-boxplot} compares translation errors based on different confidence estimation methods for inter-robot loop closures and optimization techniques during map optimization. Our proposed confidence estimation, derived from the feature correspondences ratio, significantly outperforms the commonly used uniform confidence estimates, which are often adopted due to the difficulty of accurately estimating confidence~\cite{lajoieSwarmSLAMSparseDecentralized2024}. The figure illustrates that, even with the non-robust Levenberg-Marquardt optimization~\cite{f.dellaertetal.GeorgiaTechSmoothing}, our method produces accurate results, whereas uniform confidence estimates lead to failure. Moreover, our approach achieves results comparable to the computationally expensive Graduated Non-Convexity solver~\cite{yangGraduatedNonConvexityRobust2020b}.

\ExecuteMetaData[figures/experimentation_figures.tex]{ratios-results}

In~\cref{fig:ratios-results}, we compare different correspondences ratios threshold, used for outlier rejection, with the Average Translation Error (ATE), using the LM solver with either uniform confidence or correspondences ratio-based confidence. The dashed line represents the number of loop closures at various threshold levels. A higher ratio results in a more conservative solution, yielding fewer loop closures. Notably, with our ratio-based confidence estimation, the ATE remains low even with less conservative thresholds, showing that this method simplifies parameter tuning by effectively minimizing the influence of outliers without relying on a robust solver. However, if the ratio threshold is set too conservatively, insufficient inter-robot loop closures are included, leading to decreased accuracy or failure to merge the maps.

We also observed that while our odometry-based scaling initialization sometimes improved results, it could also lead to worse performance. This suggests that our assumption—that MASt3R yields similar relative pose scales for odometry images and loop closure images—may not always hold, and altering initial estimates in local solvers can have a significant impact. Therefore, using the raw output directly and relying solely on scale optimization may offer equally good results.

Overall, these findings demonstrate the robustness and flexibility of our approach. Even with initial scale inaccuracies, the system can adapt and optimize effectively without requiring computationally expensive methods. Our independent and smoothed scale formulations consistently provide accurate results while maintaining efficient performance.
